# Supplementary material for: CoDEx: Combining Domain Expertise for Spatial Generalization in Satellite Image Analysis
Source: arXiv:2504.19737 source file (2025-04-28)
Supplement: Supplementary file 1 [file suppmat.tex]

%auto-ignore
